# Supplementary material for: Raman-acoustofluidic integrated system for single-cell analysis
Source: arXiv:2011.07520 ancillary file (2020-11-15)
Supplement: Supplementary file 1 [file Raman-acoustofluidics_ESI.pdf]

Electronic Supplementary Information (ESI)

# Raman-acoustofluidic integrated system for single-cell analysis

Harrisson D. A. Santos,[*†a] Amanda Evelyn,[*b] Giclênio C. Silva,[*a], Everton B. Lima,[a], Alisson S. Marques,[a] Magna S.Alexandre-Moreira,[b] Aline C. Queiroz,[c] Carlos Jacinto,[d] J. Henrique Lopes,[e] Ueslen Rocha,[c] and Glauber T. Silva[†a]

### S1. Acoustofluidic trapping of polystyrene beads

To investigate the arrangement behavior for trapped-polystyrene beads to the acoustic- trapping plane, a study exploring different concentrations was performed. In Fig S1, concentrations of C = 900, 400, 200 and 100 particles/µl for 10 µm-diameter polystyrene beads (dispersed in aqueous solution) were analyzed. A close-packed arrangement of a single-layer of beads in the acoustic-trapping plane, in a shape of hexagonal lattice, was observed at all concentrations. It is important to point out that, for the case of C= 900 particles/µl, some particles were concentrated at the center but somehow below the acoustic-trapping plane, whereas some other particles were already occupying that position (Fig. S1a-d). A similar arrangement was observed for 30 µm-diameter polystyrene beads, examining concentrations of C = 300, 200, 100 and 50 particles/µl. Again, single-layer hexagonal packed was settle for all concentrations explored, as shown in Fig. S2. In contrast, when higher concentrations are inspected (see the cases of C = $15\times10^3$ and $5\times10^3$ for 10 µm- and 30 µm-polystyrene beads, in Fig S4), other microparticle layers underneath the acoustic-trapping plane are observed.

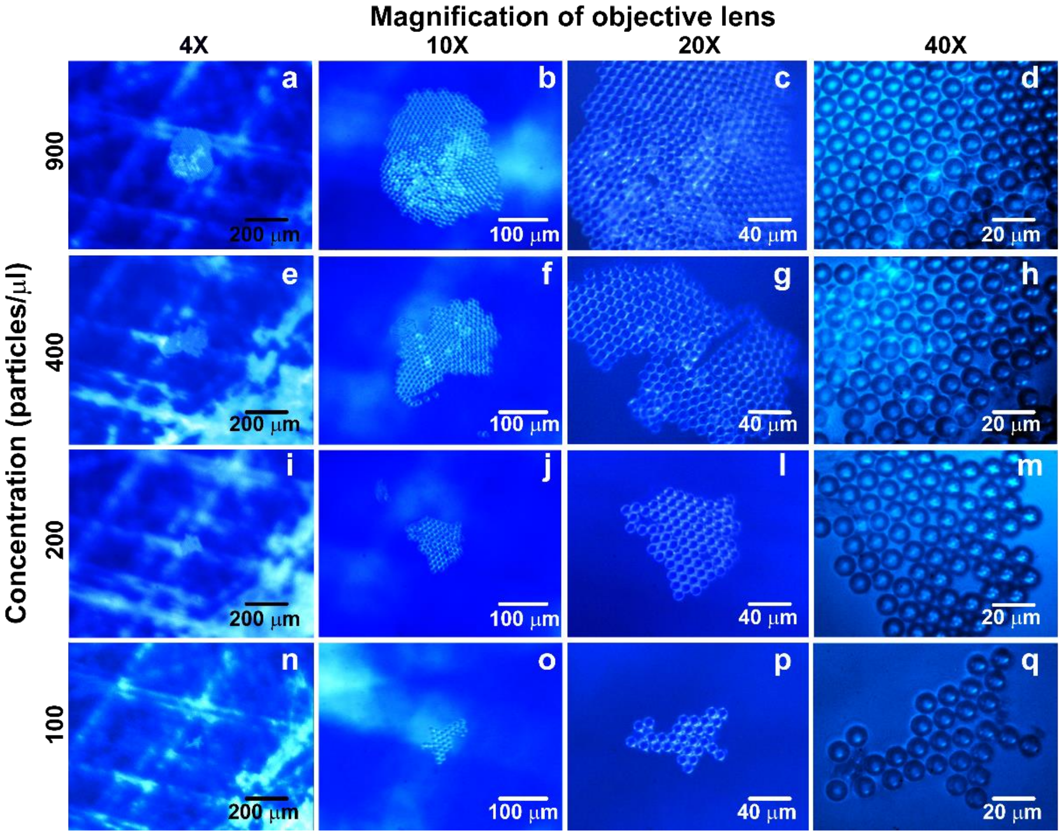


**Fig. S1.** Micrographs of monosdispersed 10 µm-diameter polystyrene dispersed in distilled water in the acoustofluidic chamber. Different concentrations of 900, 400, 200 and 100 particles/µl were inspected. The device operates at 1:056MHz with a voltage amplitude of 3:8V.

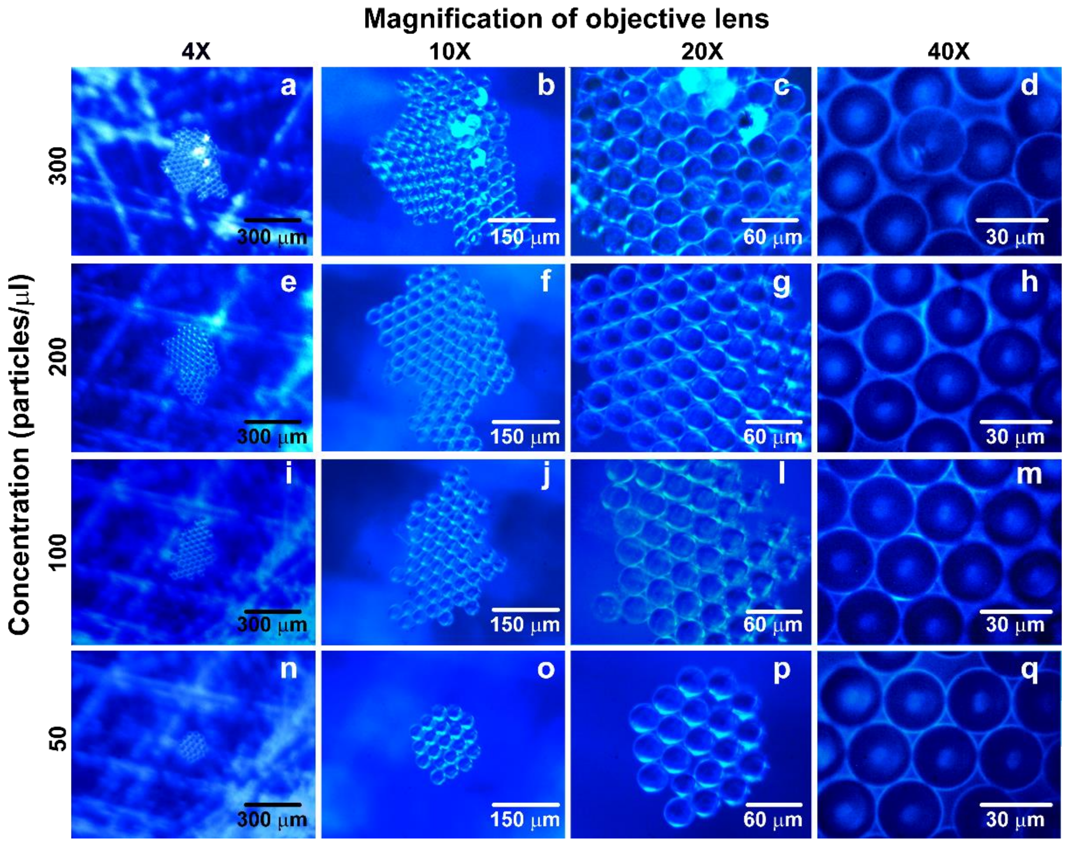


**Fig. S2.** Micrographs of monosdispersed 30 µm-diameter polystyrene beads immersed in distilled water in the acoustofluidic chamber. Different concentrations of 300, 200, 100 and 50 particles/µl were inspected. The device operates at 1:056MHz with a voltage amplitude of 3:8V.

## S2. Raman-microscanning of trapped polystyrene beads

The one-layer aspect of the trapped-beads demonstrated by optical inspection, for the cases presented in Figs. S1 and S2, were also supported by performing an axial Raman micron-scanning to them. For both size cases, 10 µm- and 30 µm-beads, a laser scanning cross-centered on a single-particle, along the axial line (from z = -80 to z= 80µm), was performed. The Raman intensity average value around the 1000cm$^{-1}$ peak of the polystyrene beads was used to assess the Raman-intensity profile along the z-axis (see Fig. S3a-h). The full width at half maximum (FWHM) of the Raman intensity profiles are around 15µm (Fig. S3i) and 33µm (Fig. S3j) for 10µm-beads and 30µm-beads, respectively, at all concentration ranges investigated. Such result corroborate to both single-layer beads-package arrangement and single-particle Raman assessment. On the other hand, for concentrations as C≥ 5×10$^{3}$particles/µL, the FWHM broadens due to the formation of other microparticle layers underneath the levitation plane (see

Fig S4). In all cases, the Raman intensity profiles were taken under 785 (2mW of laser power and 30s of acquisition time) focused through a 40×/0.65 objective lens.

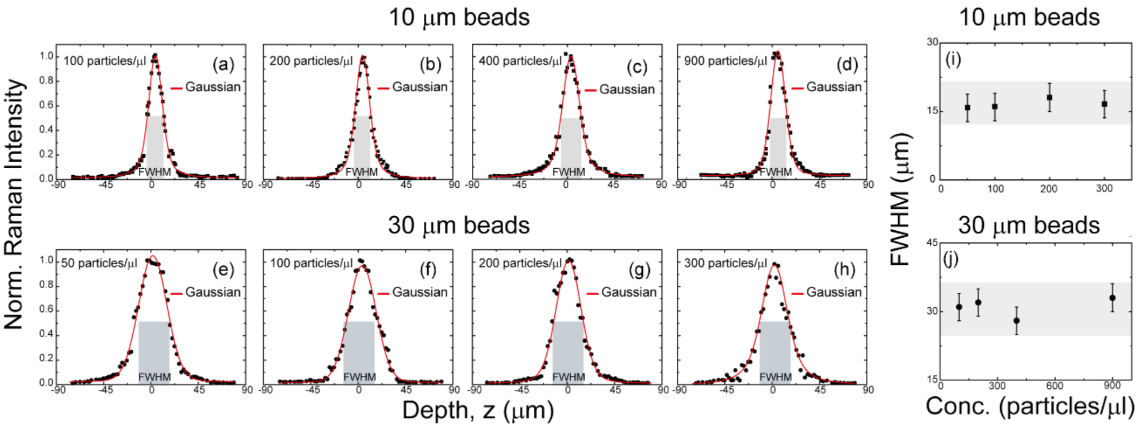


**Fig. S3.** Raman intensity profiles of the average value around the 1000cm$^{-1}$ peak of the polystyrene beads. The intensity profiles were attained through an axial laser-scanning cross-centered in a single-particle. Concentrations of (a) 100, (b) 200, (c) 400 and (d) 900 particles/µl for 10µm-beads and (e) 50, (f) 100, (g) 200 and (h) 300 particles/µl for 30µm-beads were investigated. The full width at half maximum (FWHM) of the Raman intensity profiles are around (i) 15µm and (j) 33µm for 10µm-beads and 30µm-beads, respectively, regardless of the concentration used. The red line depicts a Gaussian fit of the measured data. In all cases, the Raman intensity profiles were taken under 785 (2mW of laser power and 30s of acquisition time) focused through a 40×/0.65 objective lens.

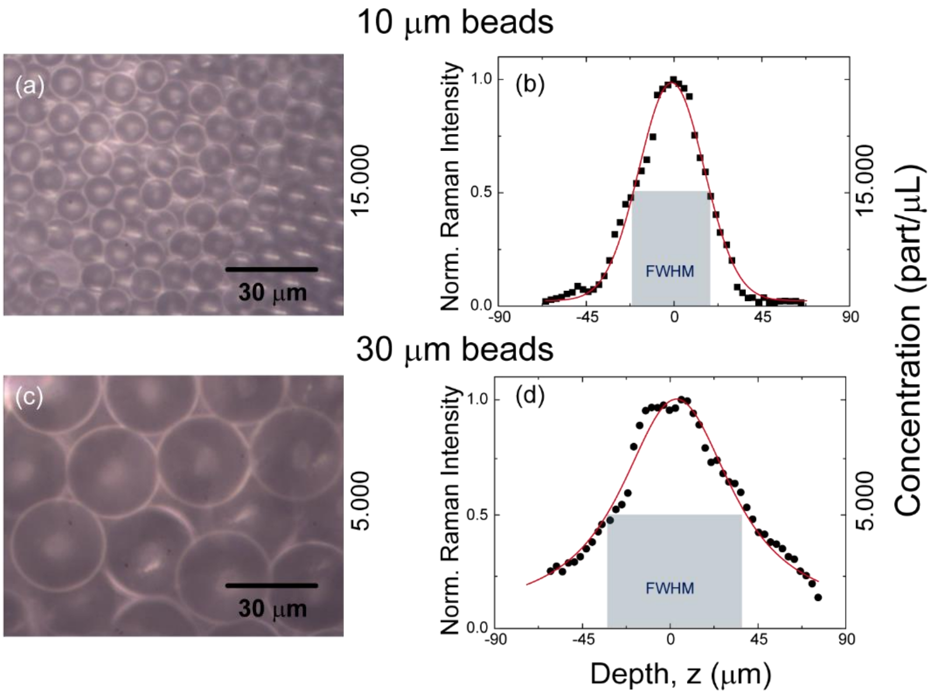


**Fig. S4. .** Bright field images of (a) 10 µm- and (c) 30 µm-polystyrene beads dispersed in distilled water in the acoustofluidic chamber**.** The concentrations employed in those cases were C = 15x10$^3$ and 5x10$^3$ particles/µl for (a) and (c), respectively. The Raman intensity profiles of the average value around the 1000cm$^{-1}$ peak for each case presented in (a) and (c) are displayed in (b) and (d), respectively. In both cases, the Raman intensity profiles were taken under 785 nm excitation (15mW of laser power and 30s of acquisition time) focused through a 40×/0.65 objective lens. The full width at half maximum (FWHM) of the Raman intensity profiles are around 40µm and 67µm for (b) and (d), respectively. The enlargement behavior of these FWHM`s, when compared to those presented in Fig. S3 (C ≤900 particles/µl), clearly show a formation of other microparticles layers

underneath those in the acoustic levitation-plane. These underneath-layers of microparticles are also easily observed by careful inspection of the optical images in (a) and (c).

## S3. Average temperature inside the acoustofluidic chamber

Temperature plays an important role in acoustofluidic features inside the acoustofluidic-chamber[1-3] as well as cellular viability[4, 5]. In order to avoid any thermal effect during the acoustic-trapping procedure, we used a low-amplitude voltage of 3.8V. Time evolution of the overall acoustofluidic-chamber temperature for different operation voltages (from 2 to 20 V) are displayed in Fig. S5a. During the measurements, the acoustofluidic-chamber contained an aqueous solution of 10 μm-polystyrene beads. For each applied voltage, the application time was 5 min, and the steady-state temperature increments reached are displayed in Fig. S5b. No remarkable variations on temperature are observed at operate voltages as low as 8V. This result suggests that effects related to voltage-induced thermal loading were avoiding as we worked in a low-voltage regime during the acoustic-trapping mechanisms. On the other hand, voltages above 10V, the voltage-induced thermal loading is evident. The acquisition thermal system used was FLIR E40 bx. This camera was remotely controlled through FLIR Tools software and had an accuracy of 0.2 ° C in the -20-120 ° C range.

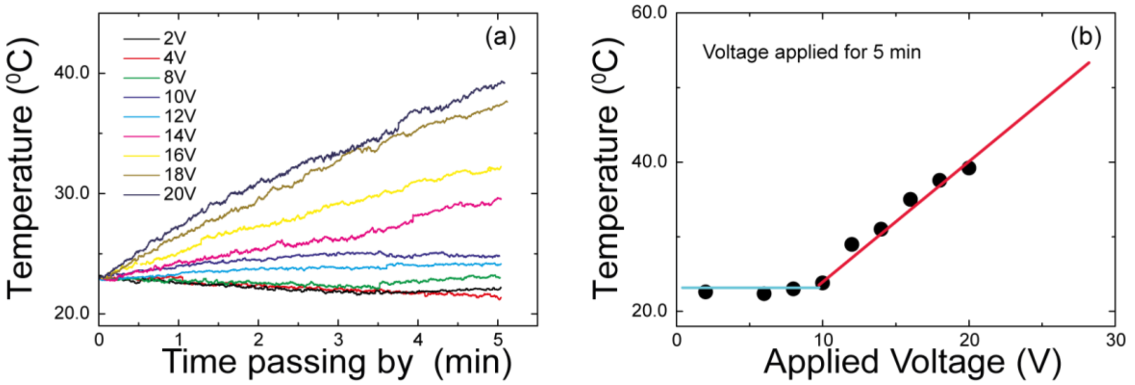


**Fig. S5.** Time evolution of the overall acoustofluidic-chamber temperature for different operation voltages (from 2 to 20 V) are displayed in (a). The acoustofluidic-chamber was filled with an aqueous solution of polysterene beads for such measurements. For each voltage, the application time was 5 min, and the steady-state temperature increments reached are displayed in (b). Remarkable temperature variations are only observed for voltages above 10 V. The acquisition thermal system used was FLIR E40 bx. This camera was remotely controlled through FLIR Tools software and had an accuracy of 0.2 ° C in the -20-120 ° C range.

## S4. Numerical simulations

Comsol Multiphysics Software (Comsol Inc., USA) was used to calculate numerically the acoustic fields inside the device chamber. The simulation parameters correspond to the actual experimental setup as given in Table S1. The device's cylindrical symmetry enabled us to use a 2D-axisymmetric model for the mesh representation of the device. The model equations and boundary conditions are based upon Refs [6, 7]. In summary, the simulation method is asfollows. (i) The electrostatic module simulates the piezoelectric ceramic excitation. (ii) The viscoelastic solids module is used for the wave propagation in the coupling mediums and acoustic reflector (resin and glass). (iii) The acoustic pressure module is employed to calculate the pressure and fluid velocity fields within the acoustofluidic chamber (See Eqs. 2a and 2b in the main text). All simulations were performed in a desktop computer (Intel Core i7-3770K CPU @ 3.50GHz, 4 cores, and 32GB of Ram) with the Linux operating system (64 bits). In Fig. S6, we show the mesh convergence plot based on the acoustic radiation force potential, $U^{rad}$ (Eq. 2a in the main text), through the expression

$$\text{Convergence (\%)} = 100\sqrt{\frac{\int (\mathrm{U^{rad}}(\mathrm{n}) - (\mathrm{U^{rad}}_{\mathrm{ref}})^{\,2}\,\mathrm{dxdz}}{\int (\mathrm{U^{rad}}_{\mathrm{ref}})^{\,2}\,\mathrm{dxdz}}} \quad \text{(S1)}$$

Where the mesh parameter *n* being the denominator of the ratio of the maximum element size finite mesh ($mesf_{max}$ = (water wavelength)/*n*) [3]. We adopted $n$ = 35, as we have an error smaller than 0.1% and a satisfactory simulation time of 30 seconds, using about 8GB of RAM. We obtained the result shown in Fig. 2 (see in the main text) after sweeping the frequency from 0.90 and to 1.1 MHz.

**Table S1. Parameters used in Comsol numerical model.**

| Description | Value |
|---|---|
| **Device** | |
| Frequency | 1.093 MHz |
| Cavity radius | 2 mm |
| Cavity height | 750 µm |
| PZT radius | 12.5 mm |
| PZT thickness | 2 mm |
| Tension application | 3.8 V |
| Device height | 5.6 mm |
| Device radius | 19 mm |
| Coverslide (glass) thickness | 150 µm |
| Coverslide (glass) radius | 16 mm |

| | |
|---|---|
| **Water** | |
| Wavelength | 1.366 mm |
| Density | 998 kg/m³ |
| Speed of sound | 1493 m/s |
| Bulk Modulus | 2.2246 GPa |
| Dynamic viscosity | 1.002 mPa·s |
| Bulk viscosity[8] | 2.87 mPa·s |
| **Polystyrene** | |
| Radius | 5 μm |
| Density | 1050 kg/m³ |
| Speed of sound | 2170 m/s |
| Shear speed | 1100 m/s |
| Bulk Modulus | 3.2503 GPa |
| **Glass** | |
| Density | 2600 kg/m³ |
| Speed of sound | 5521 m/s |
| Shear speed | 3449 m/s |
| **3D Resin parameters**[9] | |
| Density | 1107 kg/m³ |
| Longitudinal speed of sound | 2136.6 m/s |
| Shear speed of sound | 890 m/s |
| Longitudinal attenuation coefficient | 29.4734 Np/m |
| Shear attenuation coefficient (estimated[10]) | 200 Np/m |

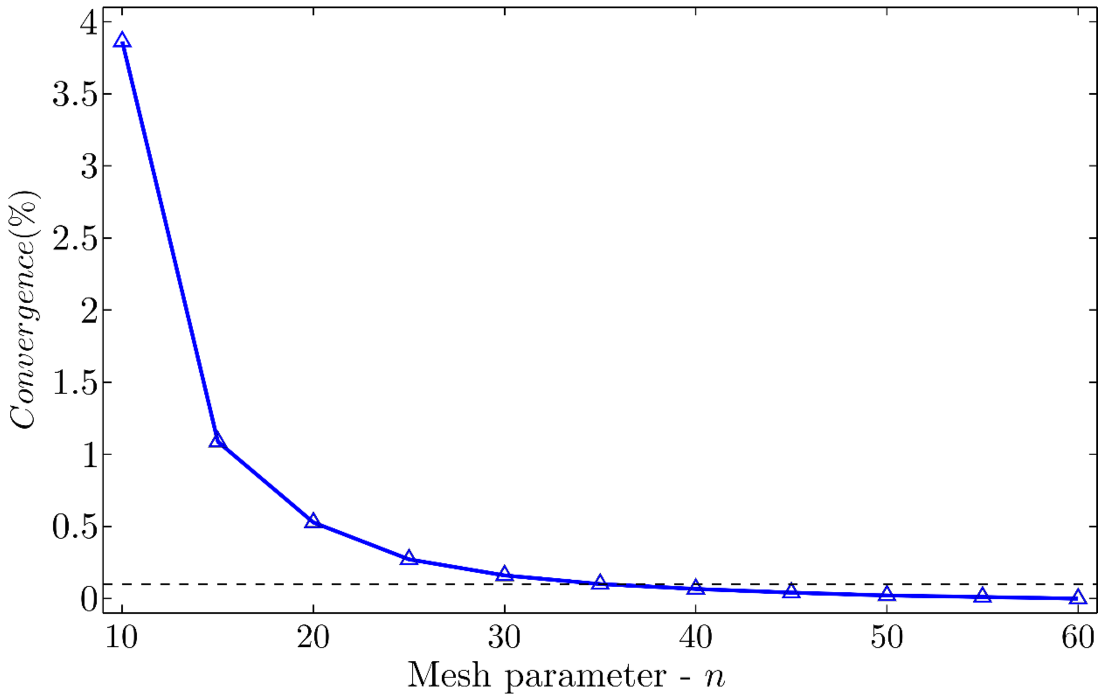


**Fig. S6**. Plot of the simulation mesh convergence, calculated from Eq. S1, with a percentage referring to the best-used mesh (*n* = 60), the dashed line refers to the chosen value, which contains a satisfactory balance between preciseness and computational time.

## Supplemental references


1. Evander, M., et al., *Noninvasive Acoustic Cell Trapping in a Microfluidic Perfusion System for Online Bioassays.* Analytical Chemistry, 2007. **79**(7): p. 2984-2991.

2. Svennebring, J., O. Manneberg, and M. Wiklund, *Temperature regulation during ultrasonic manipulation for long-term cell handling in a microfluidic chip.* Journal of Micromechanics and Microengineering, 2007. **17**(12): p. 2469-2474.

3. Augustsson, P., et al., *Automated and temperature-controlled micro-PIV measurements enabling long-term-stable microchannel acoustophoresis characterization.* Lab on a chip, 2011. **11**: p. 4152-64.

4. Reissis, Y., et al., *The effect of temperature on the viability of human mesenchymal stem cells.* Stem Cell Research & Therapy, 2013. **4**(6): p. 139.

5. Jaque, D., et al., *Nanoparticles for photothermal therapies.* Nanoscale, 2014. **6**(16): p. 9494-9530.

6. Dual, J. and T. Schwarz, *Acoustofluidics 3: Continuum mechanics for ultrasonic particle manipulation.* Lab on a Chip, 2012. **12**(2): p. 244-252.

7. Dual, J. and D. Möller, *Acoustofluidics 4: Piezoelectricity and application in the excitation of acoustic fields for ultrasonic particle manipulation.* Lab on a Chip, 2012. **12**(3): p. 506-514.

8. Holmes, M.J., N.G. Parker, and M.J.W. Povey, *Temperature dependence of bulk viscosity in water using acoustic spectroscopy.* Journal of Physics: Conference Series, 2011. **269**: p. 012011.

9. Füzesi, K. and M. Gyöngy, *Comparison of Two Inexpensive Rapid Prototyping Methods for Manufacturing Filament Target Ultrasound Phantoms.* Ultrasound Med Biol, 2017. **43**(3): p. 712-720.

10. Leão-Neto, J.P. and G.T. Silva, *Acoustic radiation force and torque exerted on a small viscoelastic particle in an ideal fluid.* Ultrasonics, 2016. **71**: p. 1-11.
